# Supplementary material for: Long-Term Optimal Delivery Planning for Replacing the Liquefied Petroleum Gas Cylinder
Source: arXiv:2112.12530 source file (2022-06-20)
Supplement: Supplementary file 1 [file appendix_jorsj.tex]

\section*{Appendix}
\section{Computational Environment Used in Field Test \label{sec:ft_computation}}
In this section, the computation environment used in field test is described (see Section~\ref{sec:field_test}).
Different computing environments were prepared for estimating the replacement date and acquiring customer lists, and determining delivery routes.
One of the following computational environments with 8-GB memory was utilized for estimating the replacement date.
\begin{itemize}
    \item Intel(R) Xeon(R) Platinum 8370C with 2.1-GHz CPU frequency
    \item Intel(R) Xeon(R) Platinum 8272CL with 2.1-GHz CPU frequency
    \item Intel(R) Xeon(R) Platinum 8171M 2.1-GHz CPU frequency
    \item Intel(R) Xeon(R) E5-2673 v4 with 2.3-GHz CPU frequency
    \item Intel(R) Xeon(R) E5-2673 v3 with 2.4-GHz CPU frequency
\end{itemize}
Moreover, one of the following computational environments with 128-GB memory was utilized for acquiring customer list'' and determining delivery route.
\begin{itemize}
    \item Intel(R) Xeon(R) Platinum 8370C with 2.1-GHz CPU frequency
    \item Intel(R) Xeon(R) Platinum 8272CL with 2.1-GHz CPU frequency
    \item Intel(R) Xeon(R) 8171M with 2.1-GHz CPU frequency
    \item Intel(R) Xeon(R) E5-2673 v4 with 2.3-GHz CPU frequency
\end{itemize}
\section{Numerical Experiment in Demand Forecast \label{sec:exp_dp}}

\subsection{Evaluation of Complementary Accuracy \label{sec:exp_polation}}
We evaluate the accuracy of $interpolation$ and $extrapolation$ of the complementary algorithm introduced in Sections~\ref{sec:complement} and ~\ref{sec:comp_NonNCU}. 
The experimental data are generated by intentionally missing the data of the target meters. 
In the {\it interpolation} experiments, we first pick up the target date, and we remove the data for $n_{\rm m}$ successive days before the target date, not including the target date. 
In the {\it extrapolation}, we remove the cumulative usages of the previous $n_{\rm m}$ successive days, including the target date.
 The two missing periods $n_{\rm m}$ are one day and 30 days and are label {\it Short} and {\it Long}, respectively. {\it Short} and {\it Long} are set because the most frequent missing interval for smart meters is one day. 
The most frequent missing interval for houses without a smart meter is 29 days.
% In addition, we added $Moderate$ as an intermediate value between $Short$ and $Long$.
In the above $4$ patterns ($2$ patterns of $interpolation$ or $extrapolation$ $\times$ $2$ patterns of $Short$ and $Long$), we experimented with four completion algorithms: Linear, Periodic, Similar, and kNN.
\subsubsection{Evaluation Settings}
% １日ごとの使用量のヒストグラム
% We show the histogram of daily gas usage in Figure xxx.
Data used for experiments are summarized as follows,
\begin{enumerate}
    \item Data : Cumulative daily meter readings (regular meter readings sent from smart meters) 
    % \begin{itemize}
    %     \item Cumulative daily meter readings (regular meter readings sent from smart meters) 
    %     \item Gas cylinder replacement data (irregular meter readings, including conventional meters)
    % \end{itemize}
    \item the Target dates $\mathcal{D}^*$ : $\{1/2/2021, 2/2/2021, \cdots, 14/3/2021\}$ ($|\mathcal{D}^*|=42$)
    \item the Target meters $\mathcal{M}^*_s$ :
    619 smart meters that have never been missing data in the target dates
    \item the Number of Missing Cumulative Usages $n_{\rm m}$ : $1$~({\it Short}) or $30$~({\it Long})
\end{enumerate}

\subsubsection{Evaluation Metrics}
For each meter $M\in \mathcal{M}_s^*$ , the evaluation metric is calculated as,
\begin{align}
\dsp \mathrm{RMSE}\,(M)= \sqrt{\frac{1}{|\mathcal{D}^*|\times (n_{\rm m}+\delta)}\sum_{D\in\mathcal{D}^*}\sum_{i=1}^{n_{\rm m}+\delta}\left(\widehat{\rm du}_{D-i}^{(M)}-{\rm du}_{D-i}^{(M)}\right)^2}
\quad
\delta =
\left\{
\begin{array}{l}
1 \quad Interpolation \\
0 \quad Extrapolation
\end{array}
\right.
\end{align}
 where the complemented daily usage is $\widehat{\rm du}_{D+i}^{(M)}$ and the actual measured daily usage is ${\rm du}_{D+i}^{(M)}$ for $M \in 
\mathcal{M}_s^*$.
% ($\delta=1$ if {\it Interpolation}, and $\delta=0$ if {\it Extrapolation})
We obtain the mean, median and maximum values after calculating the RMSE of every customer.
% \begin{enumerate}
%     \item $\dsp \mathrm{MAE}\,(M)=\frac{1}{|\mathcal{D}^*|\times N} \sum_{t=\min{\mathcal{D}^*}}^{\max{\mathcal{D}^*}}\sum_{i=t-N-\delta}^{t-\delta}\left|\widehat{\rm du}_{D+i}^{(M)}-\mu_{D+i}^{(M)}\right|$
%     \item $\dsp  \mathrm{R^2}\,(M)= 1-\frac{\dsp  \sum_{t=\min{\mathcal{D}^*}}^{\max{\mathcal{D}^*}}\sum_{i=t-N-\delta}^{t-\delta}(\widehat{\rm du}_{D+i}^{(M)}-\mu_{D+i}^{(M)})^2}{\dsp  \sum_{t=\min{\mathcal{D}^*}}^{\max{\mathcal{D}^*}}\sum_{i=t-N-\delta}^{t-\delta}(\bar{\mu}^{(M)}-\mu_{D+i}^{(M)})^2} ~  \left(\bar{\mu}^{(M)}=\frac{1}{|\mathcal{D}^*|\times N}\sum_{t=\min{\mathcal{D}^*}}^{\max{\mathcal{D}^*}}\sum_{i=t-N-\delta}^{t-\delta}{\mu_{D+i}^{(M)}}\right)$
%     \item $\dsp \mathrm{RMSE}\,(M)= \sqrt{\frac{1}{|\mathcal{D}^*|\times N}\sum_{t=\min{\mathcal{D}^*}}^{\max{\mathcal{D}^*}}\sum_{i=t-N-\delta}^{t-\delta}\left|\widehat{\rm du}_{D+i}^{(M)}-\mu_{D+i}^{(M)}\right|}$
%     \item $\dsp \mathrm{MAPE}\,(M)=\frac{100}{|\mathcal{D}^*| \times N} \sum_{t=\min{\mathcal{D}^*}}^{\max{\mathcal{D}^*}}\sum_{i=t-N-\delta}^{t-\delta}\left|\frac{\widehat{\rm du}_{D+i}^{(M)}-\mu_{D+i}^{(M)}}{\bar{\mu}}\right| ~ \left(\bar{\mu}=\frac{1}{|\mathcal{M}^*| \times |\mathcal{D}^*| \times N}\sum_{M\in\mathcal{M}^*}\sum_{t=\min{\mathcal{D}^*}}^{\max{\mathcal{D}^*}}\sum_{i=t-N-\delta}^{t-\delta}{\mu_{D+i}^{(M)}}\right)$
% \end{enumerate}
% A lower $\mathrm{MAE}$, $\mathrm{RMSE}$ and $\mathrm{MAPE}$ values are better, whereas a higher $\mathrm{R^2}$ value is better.

\subsubsection{Results and Discussion}
% The results of the experiments on completion are shown in Figure ~\ref{fig:exp1-1_in,fig:exp1-1_ex,fig:exp1-2_in,fig:exp1-2_ex,fig:exp1-3_in,fig:exp1-3_ex} and Table \ref{table:exp1-1_in},\ref{table:exp1-1_ex},fig:exp1-2_in,fig:exp1-2_ex,fig:exp1-3_in,fig:exp1-3_ex. %TODO
We show the experiment results of {\it Interpolation} in Figure~\ref{fig:exp1-1_in} and Table~\ref{table:exp1-1_in}.
These results enable us to consider the following things,

\begin{enumerate}

\item The RMSE values of Linear and Periodic are smaller than those of Similar and kNN. 
It indicates that it is more effective to use the meter's own previous data.
\item The RMSE value of Linear is equal to or lower than Periodic value because the maximum error between the measured value and the predicted value by Linear is smaller than Periodic. 
A detailed explanation is provided in Figure~\ref{fig:discussion_dp}.
%  because Linear interpolation connects the meter readings before and after the missing data with a straight line.
\end{enumerate}

Next, we show the experimental results of {\it Extrapolation} in Figure~\ref{fig:exp1-1_ex} and Table~\ref{table:exp1-1_ex}.
We also consider the following things,
\begin{enumerate}
    \item Similar and kNN shows better results than Linear and Periodic. We can see that it is more effective to use other meters' data.
    \item The RMSE value of kNN is smaller than that of Similar. It shows the effectiveness of weighting according to similarity.
    \item Although Linear has a higher RMSE value, it is expected that the risk of running out of gas is smaller because Linear uses the TQ value as the complementary value. 
    Therefore, Linear can be chosen when safety is judged to be more critical, as Section~\ref{tq complement}.
\end{enumerate}
In summary, Linear and kNN have the best accuracy in terms of Interpolation and Extrapolation complement, respectively.

% 1. 実験shortの内挿

\begin{figure}
    \centering
    \includegraphics[width=15cm]{7:Experiment_DP/figs/interpolation.png}
    \caption{Violin plot of RMSE values in the {\it interpolation}. The left table shows the results for the {\it Short} term, and the right table shows the results for the {\it Long} term.}
    \label{fig:exp1-1_in}
\end{figure}

\begin{table}[]
\begin{tabular}{crrrlcrrr}

\multicolumn{1}{c|}{Short}     & \multicolumn{1}{c|}{Mean}   & \multicolumn{1}{c|}{Median} & \multicolumn{1}{c}{Maximum} &  & \multicolumn{1}{c|}{Long}     & \multicolumn{1}{c|}{Mean}       & \multicolumn{1}{c|}{Median} & \multicolumn{1}{c}{Maximum} \\ \cline{1-4} \cline{6-9} 
\multicolumn{1}{c|}{Linear}   & \multicolumn{1}{r|}{\textbf{0.1271}} & \multicolumn{1}{r|}{\textbf{0.1142}} & 0.4716                      &  & \multicolumn{1}{c|}{Linear}   & \multicolumn{1}{r|}{\textbf{0.4028}} & \multicolumn{1}{r|}{\textbf{0.3110}} & \textbf{2.8635}                      \\
\multicolumn{1}{c|}{Periodic}   & \multicolumn{1}{r|}{0.1315} & \multicolumn{1}{r|}{0.1166} & \textbf{0.4600}                      &  & \multicolumn{1}{c|}{Periodic}   & \multicolumn{1}{r|}{0.4109} & \multicolumn{1}{r|}{0.3227} & 2.9171                      \\
\multicolumn{1}{c|}{Similar}   & \multicolumn{1}{r|}{0.1878} & \multicolumn{1}{r|}{0.1673} & 0.8658                      &  & 
\multicolumn{1}{c|}{Similar}   & \multicolumn{1}{r|}{1.4926} & \multicolumn{1}{r|}{0.9735} & 19.5941                       \\
\multicolumn{1}{c|}{kNN}   & \multicolumn{1}{r|}{0.1870} & \multicolumn{1}{r|}{0.1672} & 0.8492                      &  & 
\multicolumn{1}{c|}{kNN}   & \multicolumn{1}{r|}{1.4696} & \multicolumn{1}{r|}{0.9751} & 19.5145                      \\
\end{tabular}
\caption{The RMSE values for each complementary method during the {\it Interpolation}. The left table shows the results for the {\it Short} term, and the right table shows the results for the {\it Long} term.} 
\label{table:exp1-1_in}
\end{table}

% 2. 実験shortの外挿

\begin{figure}
    \centering
    \includegraphics[width=15cm]{7:Experiment_DP/figs/extrapolation.png}
    \caption{Violin plot of RMSE values during the {\it Extrapolation}. The left figure shows the results for the {\it Short} term, and the right figure shows the results for the {\it Long} term.}
    \label{fig:exp1-1_ex}
\end{figure}

\begin{table}[]
\begin{tabular}{crrrlcrrr}
\multicolumn{1}{c|}{Short}     & \multicolumn{1}{c|}{Mean}   & \multicolumn{1}{c|}{Median} & \multicolumn{1}{c}{Maximum} &  & \multicolumn{1}{c|}{Long}     & \multicolumn{1}{c|}{Mean}       & \multicolumn{1}{c|}{Median} & \multicolumn{1}{c}{Maximum} \\ \cline{1-4} \cline{6-9} 
\multicolumn{1}{c|}{Linear}   & \multicolumn{1}{r|}{0.2063} & \multicolumn{1}{r|}{0.1826} & 1.3320                      &  & 
\multicolumn{1}{c|}{Linear}   & \multicolumn{1}{r|}{2.5965} & \multicolumn{1}{r|}{1.7372} & 24.6073                            \\
\multicolumn{1}{c|}{Periodic}   & \multicolumn{1}{r|}{0.2588} & \multicolumn{1}{r|}{0.2280} & 1.2304                      &  & 
\multicolumn{1}{c|}{Periodic}   & \multicolumn{1}{r|}{3.9113} & \multicolumn{1}{r|}{2.9453} & 28.6447                      \\
\multicolumn{1}{c|}{Similar}   & \multicolumn{1}{r|}{0.1867} & \multicolumn{1}{r|}{\textbf{0.1671}} & 0.8757                      &  & 
\multicolumn{1}{c|}{Similar}   & \multicolumn{1}{r|}{1.4755} & \multicolumn{1}{r|}{0.9629} & 19.2096                          \\
\multicolumn{1}{c|}{kNN}   & \multicolumn{1}{r|}{\textbf{0.1860}} & \multicolumn{1}{r|}{0.1672} & \textbf{0.8579}                      &  & 
\multicolumn{1}{c|}{kNN}   & \multicolumn{1}{r|}{\textbf {1.4528}} & \multicolumn{1}{r|}{\textbf {0.9520}} & \textbf {19.1322}                                   \\
\end{tabular}
\caption{The RMSE values for each complement method during the {\it Extrapolation}. The left table shows the results for the {\it Short} term, and the right table shows the results for the {\it Long} term.}
\label{table:exp1-1_ex}
\end{table}

% \clearpage
\begin{figure}
    \centering
    \includegraphics[width=15cm]{7:Experiment_DP/figs/discussion_dp.png}
    \caption{Case in which the sum of the errors is maximum in the interpolation of Linear and Periodic. In Linear, the maximum is the gray triangle shown on the left because a straight line connects the meter readings before and after the missing data. In Periodic, the worst-case is the gray rectangle, as shown on the right. Therefore, the Periodic's maximum of the sum of errors is greater than that of Linear.}
    \label{fig:discussion_dp}
\end{figure}

\subsection{Evaluation for Forecasting Accuracy \label{sec:exp_forecast}}
The accuracy of the demand forecast presented in Sections ~\ref{sec:NCU_forecast} and~\ref{sec:NonNCU_forecast} is evaluated for meters with and without smart meters, respectively. 
As a baseline, we prepare MaxModel, which takes the maximum value of the most recent daily usage as the predicted value. Then, experiments for smart meters are compared with MaxModel, LR, SVR, RFR, and GBRT.
The coefficient of the regularization term of LR as 0.5, max depth of RFR as 4, and the other hyperparameters of each model apply the default values of sklearn \cite{scikit-learn}. 
For the experiment of conventional meters, data generation is conducted by intentionally missing the data of the target meters every 29 days. 
Thus, this is the maximum frequency of the missing data of meters without a smart meter. 
Using these data, we compare the results with MaxModel, kNN, TQ, and AllMean.

\subsubsection{Evaluation Settings}
\begin{enumerate}
    \item Data : Cumulative daily meter readings (regular meter readings sent from smart meters) 
    % \begin{itemize}
        % \item 
    %     \item Gas cylinder exchange data (irregular meter readings, including those of conventional meters) 
    % \end{itemize}
    \item the Target Dates $\mathcal{D}^*$ : $\{1/2/2021, \cdots, 14/3/2021\}$ ($|\mathcal{D}^*|=42$)
    \item the Target Meters $\mathcal{M}^*_s$ :
    619 smart meters that have never been missing data in the target dates
    \item the Number of Input Days $n_{\rm p}$: 7
    \item the Number of Samples $n_{\rm s}$ : 14
    \item the Number of Output Days $n_{\rm f}$: 9
\end{enumerate}

\subsubsection{Evaluation Metrics}
For the target date $i$, the evaluation metric is calculated as,
\begin{align*}
\dsp \mathrm{RMSE}\,(M)= \sqrt{\frac{1}{|\mathcal{D}^*|\times n_{\rm f}}\sum_{D\in\mathcal{D}^*}\sum_{i=0}^{n_{\rm f}-1}\left(\widehat{{\rm du}}_{D+i}^{(M)}-{\rm du}_{D+i}^{(M)}\right)^2}
\end{align*}
where the forecast daily usage is $\widehat{{\rm du}}_{D+i}^{(M)}$ and the actual usage is ${\rm du}_{D+i}^{(M)}$ for $M \in \mathcal{M}_s^*$.
We obtain the mean, median and maximum values after calculating the RMSE of each meter.

% \begin{enumerate}
    % \item $\dsp \mathrm{MAE}\,(M)=\frac{1}{|\mathcal{D}^*|\times L} \sum_{t=\min{\mathcal{D}^*}}^{\max{\mathcal{D}^*}}\sum_{i=t}^{t+L-1}\left|\widehat{{\rm du}}_{D+i}^{(M)}-{\rm du}_{D+i}^{(M)}\right|$
    % \item $\dsp \mathrm{R^2}\,(M)= 1-\frac{\dsp \sum_{t=\min{\mathcal{D}^*}}^{\max{\mathcal{D}^*}}\sum_{i=t}^{t+L-1}(\widehat{{\rm du}}_{D+i}^{(M)}-{\rm du}_{D+i}^{(M)})^2}{\dsp \sum_{t=\min{\mathcal{D}^*}}^{\max{\mathcal{D}^*}}\sum_{i=t}^{t+L-1}(\bar{\mu}^{(M)}-{\rm du}_{D+i}^{(M)})^2} ~ \left(\bar{\mu}^{(M)}=\frac{1}{|\mathcal{D}^*|\times L}\sum_{t=\min{\mathcal{D}^*}}^{\max{\mathcal{D}^*}}\sum_{i=t}^{t+L-1}{{\rm du}_{D+i}^{(M)}}\right)$
    % \item $\dsp \mathrm{RMSE}\,(M)= \sqrt{\frac{1}{|\mathcal{D}^*|\times L}\sum_{t=\min{\mathcal{D}^*}}^{\max{\mathcal{D}^*}}\sum_{i=t}^{t+n_{\rm f}-1}\left|\widehat{{\rm du}}_{D+i}^{(M)}-{\rm du}_{D+i}^{(M)}\right|}$
    % \item $\dsp \mathrm{MAPE}\,(M)=\frac{100}{|\mathcal{D}^*| \times L} \sum_{t=\min{\mathcal{D}^*}}^{\max{\mathcal{D}^*}}\sum_{i=t}^{t+L-1}\left|\frac{\widehat{{\rm du}}_{D+i}^{(M)}-{\rm du}_{D+i}^{(M)}}{\bar{\mu}}\right| ~  \left(\bar{\mu}=\frac{1}{|\mathcal{M}^*| \times |\mathcal{D}^*| \times L}\sum_{h\in\mathcal{M}^*}\sum_{t=\min{\mathcal{D}^*}}^{\max{\mathcal{D}^*}}\sum_{i=t}^{t+L-1}{{\rm du}_{D+i}^{(M)}}\right)$
% \end{enumerate}
% A lower $\mathrm{MAE}$, $\mathrm{RMSE}$ and $\mathrm{MAPE}$ values are better, whereas a higher $\mathrm{R^2}$ value is better.

\subsubsection{Results and Discussion}

First, we show the experimental results for smart meters on the left side of Figure~\ref{fig:NCU_forecasting} and in Table~\ref{table:NCU_forecasting}.
We consider the following things based on the results.
\begin{enumerate}
    \item The RMSE values of the four introduced models are smaller than those of the baseline MaxModel.
    \item Although the SVR and RFR are both highly accurate, the maximum value of the RMSE is the smallest for the SVR. 
    It shows that the SVR is more robust to outliers.
\end{enumerate}

Next, we show the experimental results for conventional meters on the right side of Figure~\ref{fig:NCU_forecasting} and in Table~\ref{table:NCU_forecasting}.
\begin{enumerate}
    \item The RMSE values of the proposed models are smaller than those of the baseline MaxModel.
    \item The RMSE values of the kNN are the smallest.
    It indicates that when we extract similar meters, the forecast period is also similar to that of the meters.
    \item Although TQ has a higher RMSE value, it is expected that the risk of running out of gas is smaller because TQ uses the meters' own historical third quartile as the forecast values. 
    Therefore, TQ can be chosen when safety is judged to be critical, as indicated in Section~\ref{tq complement}
\end{enumerate}

In summary, SVR/kNN achieves the highest accuracy in demand forecasts for meters with and without smart meters.

% \subsection{Result}
\begin{figure}
    \centering
    \includegraphics[width=15cm]{7:Experiment_DP/figs/forecasting.png}
    \caption{Violin plot of RMSE values in the demand forecasting. Because MaxModel records much worse results than the others, we exclude it in the figure. The left table shows the results of the demand forecast methods for smart meters, and the table on the right shows the results of the demand forecast methods for conventional meters.
    Both experiments are conducted with the smart meters because the evaluation data is quite small when we experiment with the demand forecast methods for conventional meters with the data of conventional meters.}
    \label{fig:NCU_forecasting}
\end{figure}
\begin{table}[]
\begin{tabular}{crrrlcrrr}

\multicolumn{1}{c|}{SM}     & \multicolumn{1}{c|}{Mean}   & \multicolumn{1}{c|}{Median} & \multicolumn{1}{c}{Maximum} &  & \multicolumn{1}{c|}{nonSM}     & \multicolumn{1}{c|}{Mean}       & \multicolumn{1}{c|}{Median} & \multicolumn{1}{c}{Maximum} \\ \cline{1-4} \cline{6-9} 
\multicolumn{1}{c|}{MaxModel}   & \multicolumn{1}{r|}{1.3628} & \multicolumn{1}{r|}{0.4227} & 2.165e+02                      &  & 
\multicolumn{1}{c|}{MaxModel}   & \multicolumn{1}{r|}{1.3628} & \multicolumn{1}{r|}{0.4227} & 2.165e+02                          \\
\multicolumn{1}{c|}{LR}   & \multicolumn{1}{r|}{0.5863} & \multicolumn{1}{r|}{0.4598} & 10.3792                      &  & 
\multicolumn{1}{c|}{kNN}   & \multicolumn{1}{r|}{\textbf {0.3795}} & \multicolumn{1}{r|}{\textbf {0.3478}} & \textbf {1.3350}                      \\
\multicolumn{1}{c|}{SVR}   & \multicolumn{1}{r|}{\textbf {0.3867}} & \multicolumn{1}{r|}{0.3590} & \textbf {1.4437}                      &  & 
\multicolumn{1}{c|}{TQ}   & \multicolumn{1}{r|}{0.4243} & \multicolumn{1}{r|}{0.3632} & 2.5515                      \\
\multicolumn{1}{c|}{RFR}   & \multicolumn{1}{r|}{0.3885} & \multicolumn{1}{r|}{\textbf {0.3570}} & 1.6324                      &  & 
\multicolumn{1}{c|}{AllMean}   & \multicolumn{1}{r|}{0.7722} & \multicolumn{1}{r|}{0.6084} & 4.0473                      \\
\multicolumn{1}{c|}{GBRT}   & \multicolumn{1}{r|}{0.4495} & \multicolumn{1}{r|}{0.4087} & 1.7484                      &  & 
   &      &  &                    \\
\end{tabular}
\caption{The RMSE values for each forecast model. The left table shows the results of the demand forecast methods for smart meters, and the table on the right shows the results of the demand forecast methods for conventional meters. Both experiments are conducted with the smart meters because the evaluation data is quite little when we experiment with the demand forecast methods for conventional meters with the data of conventional meters.
}
\label{table:NCU_forecasting}

\end{table}

% \clearpage
\subsection{Evaluation of Predicting the Date of Becoming High-risk Customers}

In Sections~\ref{sec:exp_polation} and~\ref{sec:exp_forecast}, the proposed models are evaluated along with RMSE.
However, when we evaluate the result of the demand forecast when considering that it is utilized for making the delivery plan, we must prepare the other evaluation metric.
Therefore, we observe how many days are different between the number of dates from becoming the high-risk houses in reality and those forecast through machine learning.

\subsubsection{Evaluation Settings}
We extract houses that do not have missing values from 1/4/2020 to 23/3/2021.
We acquire the date from when the remaining gas rate falls below the threshold of remaining gas rate in the date units. 
Then, starting from the date seven days before the date, the demand forecast and the risk function are used to calculate the date when the house becomes a high-risk house.
During the experiment, the threshold of the gas rate is set to 5\%.
In some settings, we intentionally erase the meter data by utilizing the real missing data.
We prepare the following three settings to investigate the performance of demand forecasting models, the interpolation models, and the extrapolation models.
\begin{itemize}
    \item Exp1: We utilize the complete data without intentionally making missing data. 
    Because the setting is assumed for houses with smart meters, we utilize the five demand forecast models: MaxModel(baseline), LR, SVR, RFR, and GBRT.
    \item Exp2: The data are intentionally removed based on an actual missing probability of houses with smart meters, 0.181\%. This experiment aims at determining the influence of interpolation and extrapolation. Every house is determined to become a high-risk house after interpolating the missing data. 
    Because the setting is also assumed for houses with smart meters, we utilize the same demand forecast models as Exp1.
    \item Exp3: The data are intentionally removed every 29 days. This experiment aims at determining the influence of long-term interpolation and extrapolation. 
    Because the setting is assumed for houses without smart meters, we utilize the two demand forecast models: TQ and kNN. In addition, we execute NoEx: based on the Exp3 experimental setting; we do not utilize complementing missing values but actual measurements.
\end{itemize}

\begin{figure}
    \centering
    \includegraphics[width=13cm]{7:Experiment_DP/figs/predhard/CM_7_cumulativeFalse_danger0.05_thres0.5.png}
    \caption{The result in predicting the date for becoming a high-risk house with the threshold of the integral value $\beta$ of 0.5.}
    \label{fig:predhard_0.5}
\end{figure}
\begin{figure}
    \centering
    \includegraphics[width=13cm]{7:Experiment_DP/figs/predhard/CM_7_cumulativeFalse_danger0.05_thres0.3.png}
    \caption{The result in predicting the date of becoming a high-risk customer with the threshold for an integral value $\beta$ of 0.3}
    \label{fig:predhard_0.3}
\end{figure}
\begin{figure}
    \centering
    \includegraphics[width=13cm]{7:Experiment_DP/figs/predhard/CM_7_cumulativeFalse_danger0.05_thres0.01.png}
    \caption{The result in predicting the date of becoming a high-risk customer with the threshold for an integral value $\beta$ of 0.01}
    \label{fig:predhard_0.01}
\end{figure}

\subsubsection{Results and Discussion}
The experimental results for each model are shown in Figures ~\ref{fig:predhard_0.5},~\ref{fig:predhard_0.3}, and~\ref{fig:predhard_0.01}.
Our observations are summarized as follows,
\begin{itemize}
    \item Exp1: SVR and RFR have the fewest errors in predicting the date to becoming a high-risk house, and SVR is the best when comparing the model. When the threshold for the integral value is 0.5, the distribution of the predicted days is near symmetrical.
    Therefore, some customers are predicted to be high-risk customers lately by one day compared to the correct day to be high-risk customers.
    To mitigate this situation, we can make the customer a high-risk customer earlier by decreasing the threshold $q$.
    We experimentally observe that the distribution of the days predicted to be a high-risk house is shifted earlier by one day with a threshold $q$ of 0.01. 
    Under this situation, the rate of customer prediction to be late for the actual date (particularly after seven days) decreases from 28\% to 10 \% when $q$ changes from 0.5 to 0.01.
    \item Exp2: Most of the results are the same as in Exp1, which suggests no significant influences on the prediction performance per day due to the short-term missing data.
    \item Exp3: The accuracy in predicting the date of becoming a high-risk house is not as high as Exp 1 or Exp 2 due to the fewer data acquired.
    We observe the difference by focusing on the existence of extrapolation.
    Although the actual day is most frequently observed when extrapolation is applied, a more tailed distribution of the predicted days is observed.
    The prediction result of the kNN in Exp 3 is better than LR in Exp 1 without an extrapolation, and the distribution becomes skewed.
    Therefore, an extrapolation can significantly affect the accuracy, and a demand forecast model with non-smart meters can predict the dates.
\end{itemize}

In addition, the results of the experiment on a change in threshold show that the most accurate model in each experiment is the SVR in Exp 1, SVR in Exp 2, and kNN in Exp 3, and kNN w.o. extrapolation in Exp 3, as shown in Figures~\ref{fig:predhard_exp1_svr},~\ref{fig:predhard_exp2_svr},~\ref{fig:predhard_exp3_kNN}, and~\ref{fig:predhard_exp3_kNN_NoEx}, respectively.
We can observe that customers become high-risk customers earlier as the threshold decreases.
Users can freely choose the threshold value based on these figures.

\begin{figure}
    \centering
    \includegraphics[width=13cm]{7:Experiment_DP/figs/predhard/CM_7_cumulativeFalse_danger0.05_exp1_SVR.png}
    \caption{The prediction result using SVR when changing the threshold value in Exp1}
    \label{fig:predhard_exp1_svr}
\end{figure}
\begin{figure}
    \centering
    \includegraphics[width=13cm]{7:Experiment_DP/figs/predhard/CM_7_cumulativeFalse_danger0.05_exp2_SVR.png}
    \caption{The prediction result using SVR when changing the threshold value in Exp2}
    \label{fig:predhard_exp2_svr}
\end{figure}
\begin{figure}
    \centering
    \includegraphics[width=13cm]{7:Experiment_DP/figs/predhard/CM_7_cumulativeFalse_danger0.05_exp3_kNN.png}
    \caption{The prediction result using kNN when changing the threshold value in Exp3}
    \label{fig:predhard_exp3_kNN}
\end{figure}
\begin{figure}
    \centering
    \includegraphics[width=13cm]{7:Experiment_DP/figs/predhard/CM_7_cumulativeFalse_danger0.05_exp3_kNN_NoEx.png}
    \caption{The prediction result using kNN when changing the threshold value in Exp3}
    \label{fig:predhard_exp3_kNN_NoEx}
\end{figure}

\section{Hyperparameter Tuning in Making Customer List \label{sec:appendix_dldr}}
In this section, we investigate the influence of the parameter settings for making the customer list and determining the delivery route.
\subsection{Evaluation Settings}
The replacement plans are compared when changing the parameters.
Only one parameter is changed, whereas the other parameters are fixed.
Five hours are allowed to operate our system, and the calculation is executed on the business day immediately preceding the delivery date.
The experimental settings are summarized in Table~\ref{tab:exp_result_edited}.
Numerical experiments were conducted under four different settings, as summarized in Table~\ref{tab:exp_ISG_result_edited}.
Note that when the hyperparameter $q_{\textrm{high}}$ was set to 0.5, we only focused on whether the average value of the distribution was above the threshold of the gas rate to determine a high-risk customer based on the definition of a risk function.

\subsection{Results and Discussion}
% 実験Dの結果
We use the same evaluation metrics shown in Section~\ref{sec:metric}.
The results of the evaluation metrics of the experiments are summarized in Table~\ref{tab:exp_result_edited}, enabling us to consider the following:

\begin{table}[H]
    \centering
    \begin{tabular}{c|c|c|c|c|c}
        Name & Exp 1 & Exp 2 & Exp 3 & Exp 4 & Exp 5 \\ \hline %&Exp9
        $\alpha_{\textrm{high}}, q_{\textrm{high}}$ & 5 \%, 0.3 & 5 \%, \framebox[1.1\width]{0.5} & \framebox[1.1\width]{0 \%}, 0.3 & 5 \%, 0.3 & 5 \%, 0.3 \\%& 5\%, 0.3  \\
        $\alpha_{\textrm{mdr}}, q_{\textrm{mdr}}$ & 7 \%, 0.3 & 7 \%, \framebox[1.1\width]{0.5} & 7 \%, 0.3 & 7 \%, 0.3 & 7 \%, 0.3  \\%& 7\%, 0.3  \\
        $D_{lbd}$  & 2 & 2 & 2 & \framebox[1.1\width]{0} & 2   \\%& 2  \\
        % Trip division & FAVA & FAVA & FAVA & FAVA &
        % \renewcommand{\arraystretch}{1.0}
        % \framebox[0.8\width]{\begin{tabular}{c}updated\\binpacking\end{tabular}}
        % \renewcommand{\arraystretch}{1.5} & FAVA & FAVA & FAVA  \\%& FAVA  \\
        $D_{ph}$ & 3 & 3 & 3 & 3 & \framebox[1.1\width]{0}  \\[5 pt] \hline \hline
        %Delivery Route & IP       & IP & IP & IP & IP & IP & IP & IP & TSP \\ \hline \hline
        Rate-average & 2.08 \% & -0.88 \% & -1.36 \% & 1.16 \%  & 0.49 \%  \\%&  0.83\%  \\
        Rate-median & 4.10 \% & 2.57 \% & 0.09 \% & 3.87 \%  & 2.42 \% \\
        Success & 53.3 \% & 50.1 \% & 47.1 \% & 52.5 \% &  47.7 \%  \\%& 53.0\%  \\
        Fail-out & 36.6 \% & 41.1 \% & 45.1 \% & 36.9 \% & 38.9 \%  \\%& 36.6\%  \\
        \textbf{Fail-over(↓)} & 10.1 \% & 8.7 \% & \textbf{7.8 \%} & 10.6  \% & 13.4 \%  \\%& 10.4\%  \\
        Fail-time(↓) & \textbf{0} & 1 & \textbf{0} & 1  & \textbf{0}  \\ %\hline \hline %& 0  \\
        % Number of trip & 14 & 14 & 14 & 14  & 14  \\ %& 336  \\
        % Visit(↑) & 347 & 345 & 357 & 320  & 350  \\ \hline \hline %& 336  \\
        Time/customer(↓) & 13m06s & 13m00s & 12m05s & 13m38s & 11m24s  \\%& 13m01s  \\
        Distance/customer(↓) & 1.8 km & 1.8 km & 1.5 km & 2.0 km  & 1.2 km  \\%& 43.2km  \\ commend outのvisit, number of tripより算出
        % Distance/trip(↓)& 44.7 km & 43.8 km & 37.0 km & 46.1 km  & 31.1 km  \\%& 43.2km  \\
        % Visit/day(↑) & 49.6 & 49.3 & 51.0 & 45.7  & 50.0 \\%& 48.0 \\
        \textbf{Run-out(↓)} & 28.1 & 31.6 & \textbf{21.6} & 26.6 & 29.6 \\
    \end{tabular}
    \caption{Hyperparameter settings for each experiment setting and evaluation metric of the experiment. 
    The surrounding rectangles highlight the differences in the settings between Exp 1 and the others. The best results are presented in bold.}
    \label{tab:exp_result_edited}
\end{table}

\begin{enumerate}
    \item ($\boldsymbol{q_{\textrm{high}}, q_{\textrm{mdr}}}$) The difference between Exp 1 and Exp 2 is the threshold for determining high- and moderate-risk customers.
    The experiments were conducted to observe the effect of considering the risk function defined in Section~\ref{sec:risk_func}.
    \begin{itemize}
        \item Exp 1 succeeded in increasing the success rate and decreasing the fail-out rate, but it failed to increase the fail-over rate.
        Because $q_{\textrm{high}}$ and $q_{\textrm{mdr}}$ were smaller in Exp 1, customers were more likely to be included in the customer list for replacement than in Exp 2.
        A smaller fail-out rate was observed by decreasing the parameters $q_{\textrm{high}}$ and $q_{\textrm{mdr}}$, which shows the effectiveness of considering the risk function described in Section~\ref{sec:risk_func}.
    \end{itemize}
    \item ($\boldsymbol{\alpha_{\textrm{high}}}$) In Exp 3, the remaining gas rate was set to 0\%, whereas it was set to as 5\% in Exp 1.
    \begin{itemize}
        \item Fewer run-out and fail-over events were observed in Exp 3 compared with Exp 1.
        Because $\alpha_{\textrm{high}}$ was smaller in Exp 3, it was possible to focus more on delivering to a customer who was about to experience a run-out event than with Exp 1.
        In other words, Exp 1 was more likely to achieve visit to customers whose remaining gas was not below 0\%, even if they were high-risk customers.
        The results indicate that we can focus on delivering to customers with a specific gas rate by changing $\alpha_{\textrm{high}}$.
    \end{itemize}
    \item (\textbf{$\boldsymbol{D_{lbd}}$}) Exp 4 did not force the addition of more moderate-risk customers without considering $D_{lbd}$, aiming to reveal the effectiveness of such dates.
    \begin{itemize}
        \item $D_{lbd}$ makes the number of moderate-risk customers increased.
        Notably, some customers were in the moderate-risk group in Exp 1. 
        However, they were not moderate-risk customers in Exp 4.
        These customers enabled us to obtain a smaller delivery area than in Exp 4.
        Such customers even had a low risk of experiencing a gas shortage.
        Therefore, more run-out events in Exp 1 were reported, with a larger number of visits and shorter distances/trips.
        However, for few high- and moderate-risk customers, we can obtain more candidates for visit to replace cylinders by setting $D_{lbd}$ larger than zero.
	This is a promising technique for realizing workload leveling.
        \item The two systems were competitive with respect to all evaluation metrics.
        This indicates that the influence of changing the trip division is slight when compared with the other parameters.
    \end{itemize}
    \item (\textbf{$\boldsymbol{D_{ph}}$}) The planning horizon was set to three and zero, in Exp 1 and Exp 5, respectively.
    \begin{itemize}
        \item In Exp 5, distance/customer was shorter than in Exp 1 because minimizing the delivery area for multiple days was not implemented when formulating the customer list for replacement. As a result, although problems to acquire customer lists in both Exp 1 and Exp 5 provide optimal solutions, the customer list of the first day in Exp 5 is equal to or smaller than that in Exp 1. Therefore, Exp 1 recorded worse results than Exp 5 regarding time/customer and distance/customer.
    \end{itemize}
    In conclusion, Exp 3 achieved the best results in fail-over and run-out events and had the best hyperparameter settings between Exp 1 and Exp 5.
\end{enumerate}

\section{Ablation Study on the Formulation to Acquire Customer List \label{sec:exp_ablation}}
The formulations of the proposed methods and when the depot need not be included in the rectangle, such as the formulation in~\cite{baller2019dynamic}, were compared.
The hyperparameter settings followed by Exp 3 are described in Appendix~\ref{sec:appendix_dldr}.
\begin{wrapfigure}[18]{r}[3mm]{0.7\linewidth}
% \begin{figure}[htbp]
    \centering
    \includegraphics[width=\linewidth]{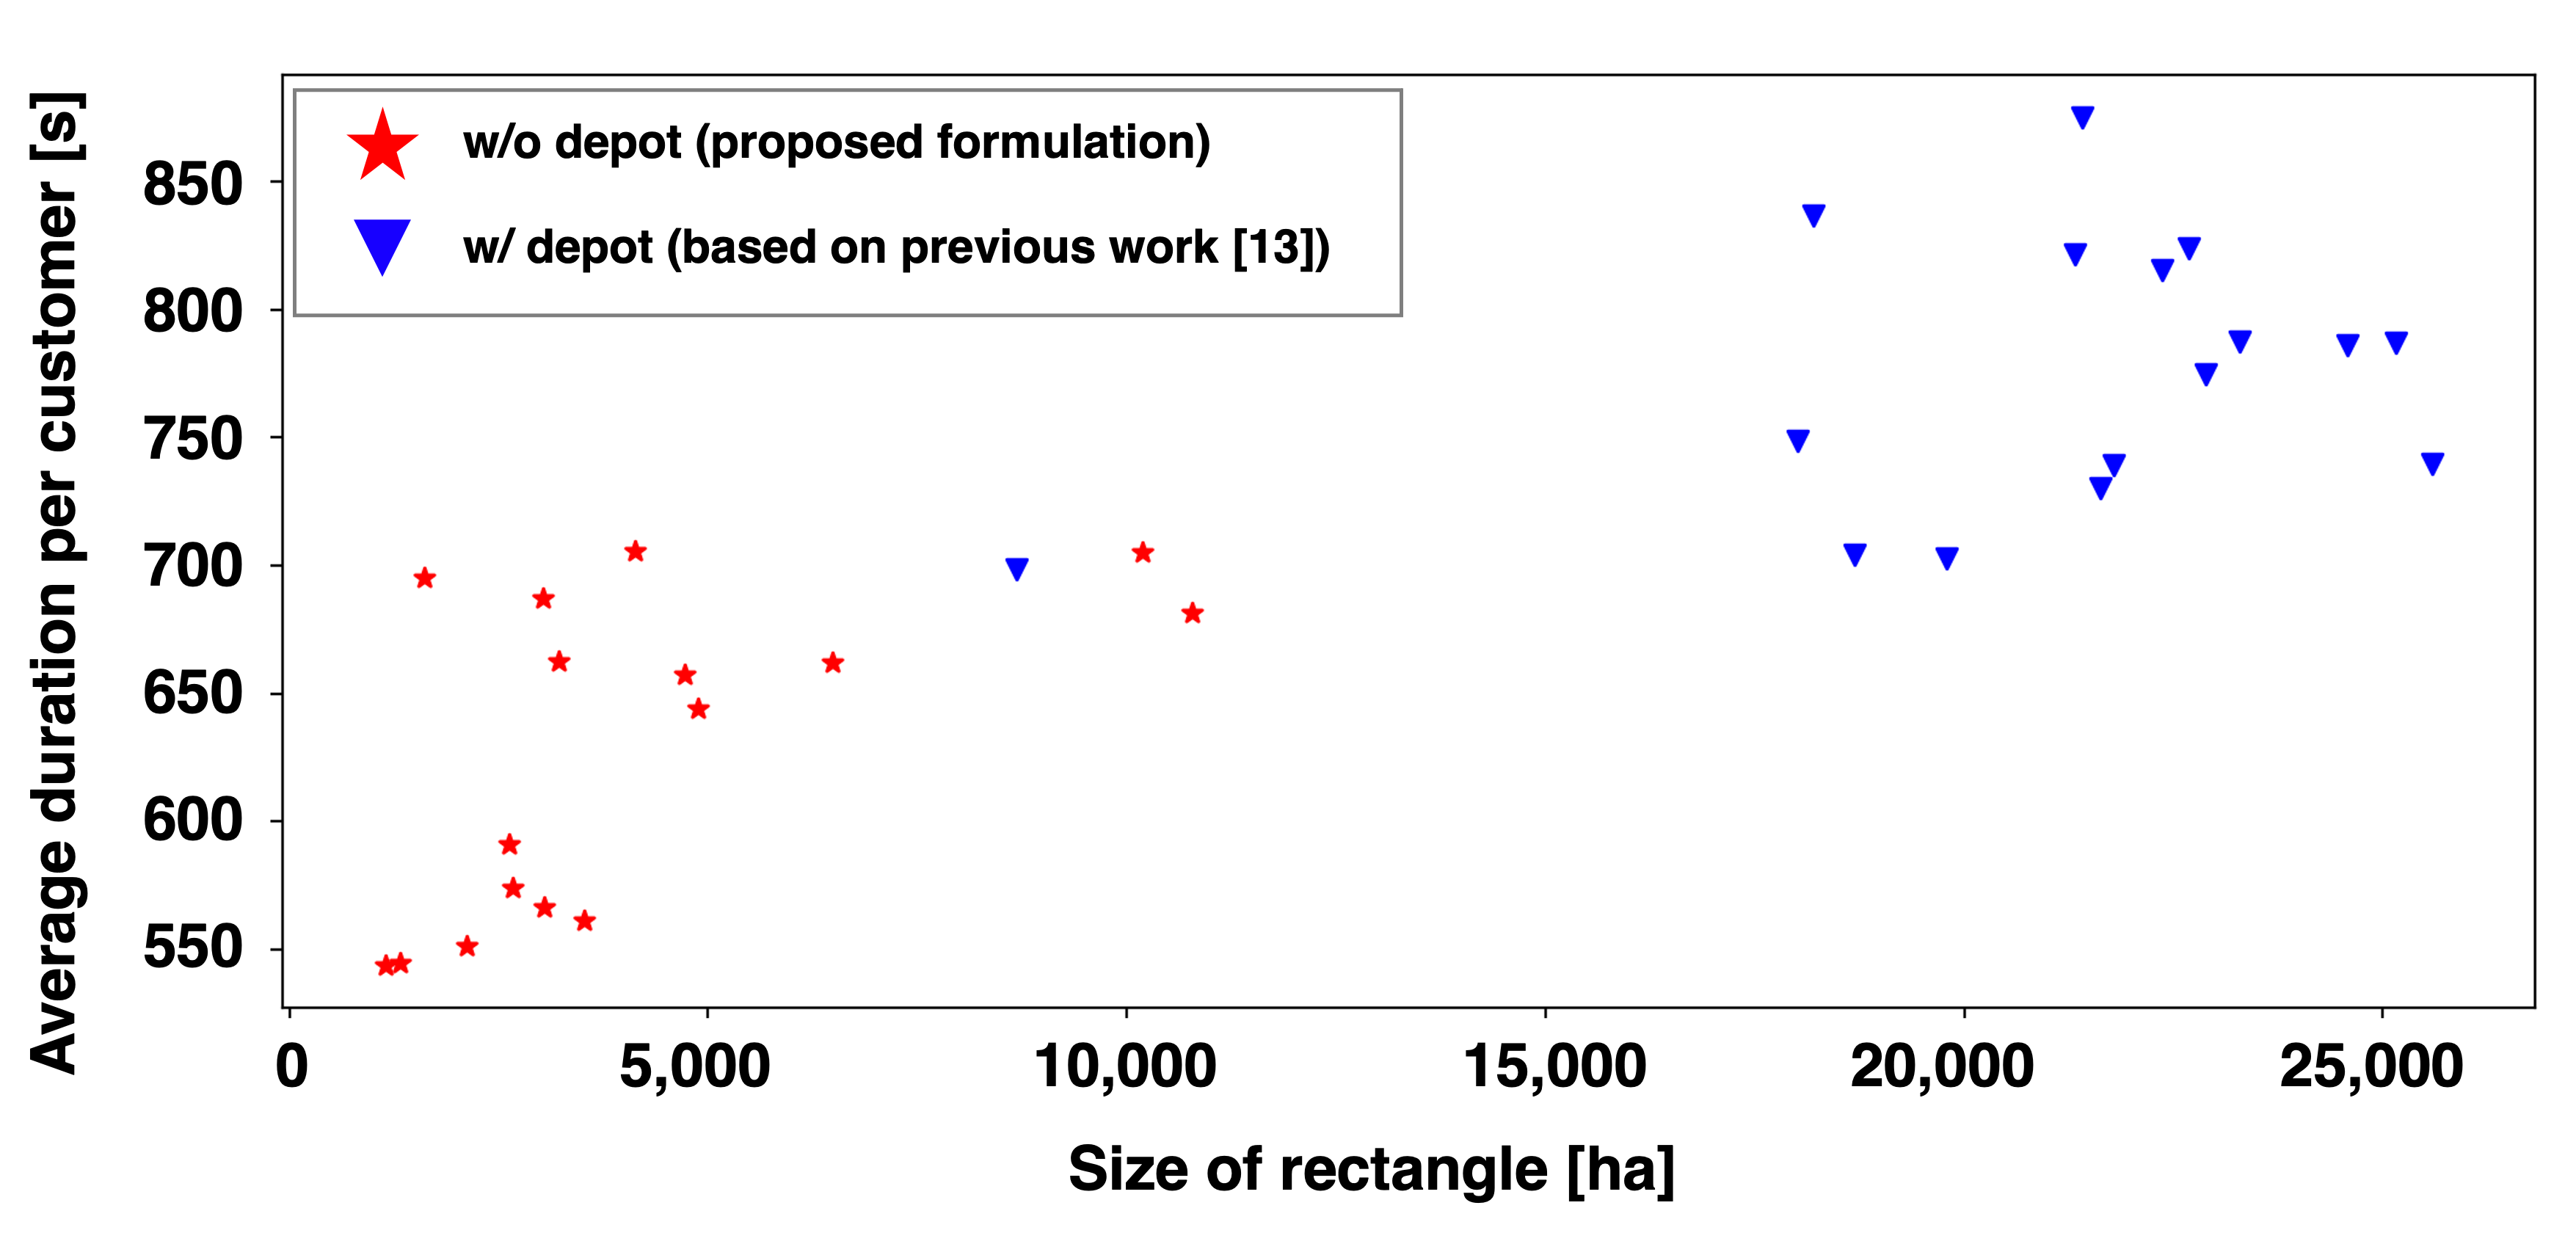}
    \caption{Scatter plot of the size of rectangle obtained by solving Problem~\ref{prob:multiBB} and average duration of delivery per customer. Blue triangle markers represent the result from an addition constraint in which the depot must be covered by a rectangle.}
    \label{fig:ablation}
% \end{figure}
\end{wrapfigure}
Figure~\ref{fig:ablation} shows the pairing of the size of the rectangle and the average delivery time, and each dot represents a trip.
With both methods, the size of the rectangle represented the cost of geographical delivery costs, and in fact, there was a correlation with respect to the average duration per customer.

From Figure~\ref{fig:ablation}, we can see that the average duration per customer for the proposed system (without depot) was smaller than that of the method in \cite{baller2019dynamic} (with depot).
This indicates that the proposed method acquires a more efficient delivery route.
This is because the depot is far from the center of gravity of the customers.
When a customer far from the depot must be delivered to, the rectangle covering the depot and the customer has already covered most of the other customers.
